# Supplementary material for: TAPS Responsibility Matrix: A tool for responsible data science by design
Source: arXiv:2302.01041 source file (2023-02-02)
Supplement: Supplementary file 3 [file Appendix_A_old.pdf]

| <b>Order</b> | <b>Question</b>                                                                                                                                                                                                                                                                                                                                                                                                                                                                                                                                                                                            | <b>Component</b> | <b>Scope</b> |
|--------------|------------------------------------------------------------------------------------------------------------------------------------------------------------------------------------------------------------------------------------------------------------------------------------------------------------------------------------------------------------------------------------------------------------------------------------------------------------------------------------------------------------------------------------------------------------------------------------------------------------|------------------|--------------|
| 1            | Who is involved in this project? e.g. researchers, organizations, end users                                                                                                                                                                                                                                                                                                                                                                                                                                                                                                                                | transparency     | agents       |
| 2            | What the outputs or deliverables of the project are? e.g. types of data to collect/re-use, models or algorithms                                                                                                                                                                                                                                                                                                                                                                                                                                                                                            | transparency     | objects      |
| 3            | What tools or processes make those outputs or deliverables (including data science lifecycle and project planning)? e.g. data collection, cleaning, data management                                                                                                                                                                                                                                                                                                                                                                                                                                        | transparency     | process      |
| 4            | What outcomes and impacts the project will have in the world? What are the intended aims of the project? What is the intended impact?                                                                                                                                                                                                                                                                                                                                                                                                                                                                      | transparency     | impact       |
| 5            | Have all the humans involved in the project been identified? This includes data scientists, downstream users of data science objects, & data subjects (e.g., patients).<br>Are there formal agreements or explicitly described relationships between them?<br>Examples of formal agreements: employment contracts (specifically length of contract, percentage of work, employee classifications, & other characteristics that might interact with ACCOUNTABILITY), consent forms, ethical approvals, intellectual property protocols, patents, non-disclosure agreements, contracts governing engagements | transparency     | agents       |
| 6            | Are these formal agreements accessible by all of the actors?                                                                                                                                                                                                                                                                                                                                                                                                                                                                                                                                               | transparency     | agents       |
| 7            | Have the contributions of the humans who are involved been described?                                                                                                                                                                                                                                                                                                                                                                                                                                                                                                                                      | transparency     | agents       |
| 8            | Are there mechanisms in place to mitigate potential conflicts?                                                                                                                                                                                                                                                                                                                                                                                                                                                                                                                                             | transparency     | agents       |
| 9            | Is there a provision for continuity and sustainability of the project and its resources over time? (e.g., do contact emails go to institutional email addresses, not individuals'?)                                                                                                                                                                                                                                                                                                                                                                                                                        | transparency     | agents       |
| 10           | Have all data/metadata/algorithms been described [this may be a link to a document]                                                                                                                                                                                                                                                                                                                                                                                                                                                                                                                        | transparency     | objects      |
| 11           | How will you make data and algorithms you used in the analysis transparent?                                                                                                                                                                                                                                                                                                                                                                                                                                                                                                                                | transparency     | objects      |
| 12           | How will you make data and algorithms that you used in the analysis accessible to others? (such as following the FAIR principles, meeting Open Science guidelines)                                                                                                                                                                                                                                                                                                                                                                                                                                         | transparency     | objects      |
| 13           | Is any metadata given for the dataset?                                                                                                                                                                                                                                                                                                                                                                                                                                                                                                                                                                     | transparency     | objects      |
| 14           | Which algorithms/tools were used for analysis (if known)?                                                                                                                                                                                                                                                                                                                                                                                                                                                                                                                                                  | transparency     | objects      |
| 15           | Are your data and metadata in a repository? (provide links such as Github, Zenodo etc.)                                                                                                                                                                                                                                                                                                                                                                                                                                                                                                                    | transparency     | objects      |
| 16           | Are the data and metadata publicly available?                                                                                                                                                                                                                                                                                                                                                                                                                                                                                                                                                              | transparency     | objects      |
| 17           | What is the licence associated with the data?                                                                                                                                                                                                                                                                                                                                                                                                                                                                                                                                                              | transparency     | objects      |
| 18           | What is the quality of the data?                                                                                                                                                                                                                                                                                                                                                                                                                                                                                                                                                                           | transparency     | objects      |
| 19           |                                                                                                                                                                                                                                                                                                                                                                                                                                                                                                                                                                                                            |                  |              |

|    |                                                                                                                                            |              |         |
|----|--------------------------------------------------------------------------------------------------------------------------------------------|--------------|---------|
| 20 | What is the quantity of missing values in the data?                                                                                        | transparency | objects |
| 21 | Are there any terms and conditions specified on the use of the data/algorithm?                                                             | transparency | objects |
| 22 | How will you collect the data?                                                                                                             | transparency | process |
| 23 | How do you clean/preprocess the data?                                                                                                      | transparency | process |
| 24 | How do you analyze the data?                                                                                                               | transparency | process |
| 25 | Are all of the goals of the project accessible and understandable by all of the actors?                                                    | transparency | process |
| 26 | How do you maintain/serve the project or your data?                                                                                        | transparency | process |
| 27 | Within subcomponents of a process, are data FAIR?                                                                                          | transparency | impact  |
| 28 | Can you describe the implications of the project so that it is understandable by everyone?                                                 | transparency | impact  |
| 29 | Can you articulate how this project will affect people's life or research?                                                                 | transparency | impact  |
| 30 | Have you described how this project might be misused?                                                                                      | transparency | impact  |
| 31 | Are there any terms and conditions specified on the use of data/algorithm?                                                                 | transparency | impact  |
| 32 | Is there an informed consent form signed by the human subjects in the project?                                                             | privacy      | agents  |
| 33 | Has a confidentiality agreement or non disclosure agreement been signed (if applicable)?                                                   | privacy      | agents  |
| 34 | Has a data usage agreement been signed by the researchers involved?                                                                        | privacy      | agents  |
| 35 | Has a privacy protection method been used to make the data anonymous or pseudonymous?                                                      | privacy      | objects |
| 36 | Are you collecting identifiable personal information?                                                                                      | privacy      | objects |
| 37 | Are you collecting sensitive data (as defined by GDPR)                                                                                     | privacy      | objects |
| 38 | Are the data you collected necessary to answer your research questions?                                                                    | privacy      | objects |
| 39 | Where/how do you process the data? (do you upload data to some servers to execute processing? Which tools do you use?)                     | privacy      | objects |
| 40 | Where do you store data during and after your project?                                                                                     | privacy      | objects |
| 41 | Is it secure?                                                                                                                              | privacy      | objects |
| 42 | Did you do your data management plan or use a template (such as <a href="https://dmponline.dcc.ac.uk/">https://dmponline.dcc.ac.uk/</a> )? | privacy      | objects |
| 43 | Can third parties use the data? if so, how?                                                                                                | privacy      | objects |
| 44 | Do your models and results reveal personal information directly?                                                                           | privacy      | objects |
| 45 | Can the outcome can be used to identify individuals indirectly?                                                                            | privacy      | objects |

|    |                                                                                                                                                                             |                |         |
|----|-----------------------------------------------------------------------------------------------------------------------------------------------------------------------------|----------------|---------|
| 46 | Is it possible that other people can combine your model/algorithm with other resources to identify individuals?                                                             | privacy        | objects |
| 47 | Do participants have full control over their data?                                                                                                                          | privacy        | objects |
| 48 | Can they withdraw from the study at any point in time?                                                                                                                      | privacy        | objects |
| 49 | Can they provide consent for secondary re-use of the data?                                                                                                                  | privacy        | objects |
| 50 | Has a distributed learning method, such as the personal health train, been used where the algorithm is sent to the data provider and not the other way around?              | privacy        | process |
| 51 | Has the analysis been conducted on the individual or on the group level?                                                                                                    | privacy        | process |
| 52 | Has an information management system been set in place for auditing purposes?                                                                                               | privacy        | process |
| 53 | Does your project help individuals protect their privacy and confidentiality?                                                                                               | privacy        | impact  |
| 54 | Does your project increase society's confidence and trust in data science projects?                                                                                         | privacy        | impact  |
| 55 | Will your outcome deliver a positive message to people about how their privacy and confidentiality have been handled?                                                       | privacy        | impact  |
| 56 | Has the researcher signed a code of conduct agreement?                                                                                                                      | accountability | agents  |
| 57 | Is it clear who is responsible for which part of the analysis outcome?                                                                                                      | accountability | agents  |
| 58 | Does your organisation have protocols and procedures for dealing with an intentional or unintentional breakdown of transparency, privacy/confidentiality, or norm breaking? | accountability | agents  |
| 59 | Are there protocols and procedures for dealing with conflicts between legal and ethical positions in projects?                                                              | accountability | agents  |
| 60 | Does your organisation have a data protection officer? Data ethics review committees? Data stewards?                                                                        | accountability | agents  |
| 61 | Do employees have access to resources (e.g., training) for doing responsible data science?                                                                                  | accountability | agents  |
| 62 | Do protections exist against lawsuit or damages for individual data scientists, users, or organisations?                                                                    | accountability | agents  |
| 63 | Has provenance been presented to track the origin of the data?                                                                                                              | accountability | objects |
| 64 | Do you know the original permissions attached to the data (in the case of re-use)?                                                                                          | accountability | objects |
| 65 | Are you following the original permissions that are attached to that data?                                                                                                  | accountability | objects |
| 66 | Is there a description provided about potential biases, such as confounding factors?                                                                                        | accountability | objects |
| 67 | Is data quality an issue? If yes, what is the specific issue and how is it resolved?                                                                                        | accountability | objects |
| 68 | Is there a threshold for missing values? Is there a mechanism for reacting to missed thresholds?                                                                            | accountability | objects |
| 69 | Is there a clear and transparent description of the process that is accessible?                                                                                             | accountability | process |

|    |                                                                                                                                     |                 |         |
|----|-------------------------------------------------------------------------------------------------------------------------------------|-----------------|---------|
| 70 | Who is responsible for which part of the analysis?                                                                                  | accountability  | process |
| 71 | Is there any control/checkpoints within the process?                                                                                | accountability  | process |
| 72 | What is the impact or the outcome of the analysis?                                                                                  | accountability  | impact  |
| 73 | Is the outcome of your project understandable by others?                                                                            | accountability  | impact  |
| 74 | How are unintended outcomes communicated to the relevant organisation?                                                              | accountability  | impact  |
| 75 | Are there protocols and procedures for dealing with conflicts between legal and ethical positions in projects?                      | accountability  | impact  |
| 76 | Is there a procedure for dealing with unintended outcomes, either positive or negative?                                             | accountability  | impact  |
| 77 | How does your organisation deal with evaluations by external parties about the responsibility aspects of the project?               | accountability  | impact  |
| 78 | What are the operative social values and norms that touch on who is involved in the project and how their roles are governed?       | societal values | agents  |
| 79 | What are the operative social values and norms that touch on data, algorithms, and other outputs or deliverables of the project?    | societal values | objects |
| 80 | What are the operative social values and norms that touch on research processes and the data science lifecycle?                     | societal values | process |
| 81 | What are the operative social values and norms that touch on the intended and unintended consequences and outcomes of your project? | societal values | impact  |
| 82 | Do the operative social values and norms conflict with each other?                                                                  | societal values | impact  |
| 83 | Are all of the operative social values and norms in agreement with each other?                                                      | societal values | impact  |
